# Supplementary material for: Applications of Computational Topology to Fusion Science
Source: arXiv:2410.18128 source file (2024-10-17)
Supplement: Supplementary file 1 [file AppendixB.tex]

% Appendix Template

\chapter{Derivation of the separatrix map} % Main appendix title

\label{AppendixB}

%----------------------------------------------------------------------------------------
%	SECTION 1
%----------------------------------------------------------------------------------------

%----------------------------------------------------------------------------------------
%	SECTION 2
%----------------------------------------------------------------------------------------
